# Supplementary material for: Phase Competition in HfO$_2$ with Applied Electric Field from First Principles
Source: arXiv:2009.09569 ancillary file (2020-09-26)
Supplement: Supplementary file 1 [file Supplementary_Materials.pdf]

# Supplementary Materials

Yubo Qi, and Karin M. Rabe
Department of Physics & Astronomy, Rutgers University,
Piscataway, New Jersey 08854, United States

## I. COMPUTED STRUCTURAL PARAMETERS

TABLE S1. Computed structural parameters for $HfO_2$ in the $P4_2/nmc$ tetragonal structure. The lattice constants are $a = 3.465$ Å, $b = 3.465$ Å, and $c = 4.95$ Å. The lattice vectors of the 12–atom conventional unit cell referred to in the main text are obtained from these primitive lattice vectors by $(\mathbf{a}', \mathbf{b}', \mathbf{c}') = (\mathbf{c}, \mathbf{a} + \mathbf{b}, \mathbf{a} - \mathbf{b})$

| $P4_2/nmc$ | $x$ | $y$ | $z$ |
|---|---|---|---|
| Hf(2a) | 0.750 | 0.250 | 0.750 |
| O(4d) | 0.250 | 0.250 | 0.466 |

TABLE S2. Computed structural parameters for the $Pca2_1$ oIII structure. The lattice constants are $a = 5.06$ Å, $b = 4.89$ Å, and $c = 4.90$ Å.

| $Pca2_1$ | $x$ | $y$ | $z$ |
|---|---|---|---|
| Hf(4a) | 0.466 | 0.230 | 0.000 |
| O(4a) | 0.129 | 0.424 | 0.132 |
| O(4a) | -0.239 | 0.043 | 0.249 |

TABLE S3. Computed structural parameters for the $Pnm2_1$ oIV structure. Here, $a = 3.307$ Å, $b = 4.963$ Å, and $c = 3.684$ Å. The lattice vectors of the 12–atom conventional unit cell referred to in the main text are obtained from the primitive lattice vectors by $(\mathbf{a}', \mathbf{b}', \mathbf{c}') = (\mathbf{b}, \mathbf{a} + \mathbf{c}, \mathbf{a} - \mathbf{c})$.

| $Pnm2_1$ | $x$ | $y$ | $z$ |
|---|---|---|---|
| Hf(2a) | 0.000 | 0.264 | 0.000 |
| O(2a) | 0.000 | 0.448 | 0.506 |
| O(2a) | 0.000 | -0.066 | 0.660 |

TABLE S4. Comparison between the lattice constants for various $HfO_2$ phases given by this work and previous works. The calculated lattice constants with LDA functional in this work are identical with those in the previous study [S1]. All the discussions in the main text are based on the LDA results of this work, unless explicitly stated otherwise. The unit of lattice constant is Å, and the unit of energy is meV per formula unit.

| Phase | Latt. | This work[a] | This work[b] | Prev. work[c] | Prev. work[d] | Prev. work[e] | Prev. work[f] |
|---|---|---|---|---|---|---|---|
| cubic | $a$ | 4.89 | 5.04 | 5.04 | 5.25 | 5.04 | - |
| | $E$ | 105.0 | 279.1 | - | - | - | - |
| tetragonal | $a'$ | 4.95 | 5.20 | 5.13 | 5.37 | 5.11 | 5.28 |
| | $b' = c'$ | 4.90 | 5.04 | 5.06 | 5.30 | 5.03 | 5.06 |
| | $E$ | 80.2 | 166.5 | - | - | - | - |
| oIII | $a$ | 5.06 | 5.24 | - | - | 5.29 | |
| | $b$ | 4.89 | 5.01 | - | - | - | 5.01 |
| | $c$ | 4.90 | 5.05 | - | - | - | 5.08 |
| | $E$ | 49.8 | 90.5 | - | - | - | - |
| oIV | $a'$ | 4.98 | 5.08 | - | - | - | 5.18 |
| | $b'$ | 4.95 | 5.16 | - | - | - | 5.13 |
| | $c'$ | 4.95 | 5.16 | - | - | - | 5.13 |
| | $E$ | 110.2 | 151.9 | - | - | - | - |
| monoclinic | $a$ | 5.08 | 5.29 | 5.28 | 5.37 | 5.22 | 5.31 |
| | $b$ | 5.06 | 5.15 | 5.17 | 5.40 | 5.19 | 5.20 |
| | $c$ | 4.95 | 5.10 | 5.11 | 5.29 | 5.08 | 5.14 |
| | $\beta$ | 99.53° | 80.3° | 99.35° | 97.92° | 99.77° | 99.8° |
| | $E$ | 0 | 0 | - | - | - | |

[a] LDA functional

[b] GGA functional

[c] LDA functional, Reference [S2]

[d] GGA functional, Reference [S2]

[e] LDA functional, Reference [S3]

[f] GGA functional, Reference [S4]

## II. SYMMETRY-ADAPTED LATTICE MODES FOR THE CUBIC FLUORITE STRUCTURE

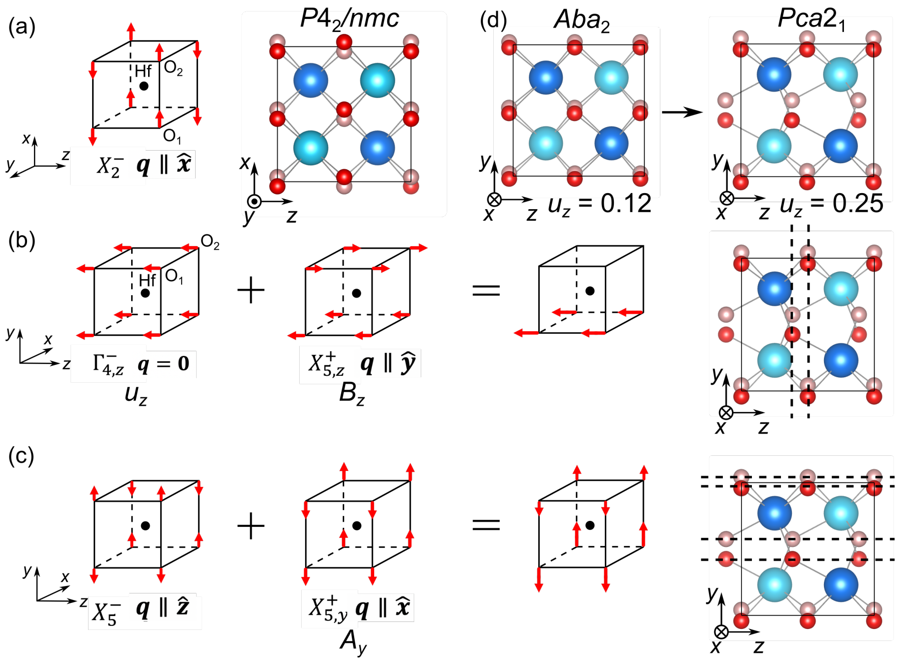


FIG. S1. (a) The anti–polar $X_2^-$ mode generates the $P4_2/nmc$ structure. The axis orientation here is different from that in other sub–figures for clarity. (b) Polar $\Gamma_{4,z}^-$ and anti–polar $X_{5,z}^+$ modes combine to generate the $Pca2_1$ structure from the $P4_2/nmc$ structure. The amplitude of the $X_{5,z}^+$ mode ($B_z$) determines the difference in $z$–direction displacements of the oxygen atoms in neighboring layers. Destructive interference of these two modes leads to zero displacement for half of the layers of oxygen atoms. (c) Anti–polar $X_{5,y}^+$ and $X_5^-$ modes are symmetry–allowed in the $Pca2_1$ structure. The amplitude of the $X_{5,y}^+$ mode ($A_y$) determines the difference in separation of oxygen atoms along the $y$ direction in neighboring layers. The layers with a larger separation results from the constructive interference of the two modes, and the layer with a smaller one results from the destructive interference. (d) Structural change as $u_z$ increases; For $0 < u_z \leq 0.12$ Å (the Hf atoms are slightly displaced to the right), the structure has a $Aba_2$ symmetry, with $A_y \neq 0$ and $B_z = 0$. It can be seen in the structure that the oxygen atoms separate along the $y$ axis, but have the same displacements along the $z$ axis. For $u_z > 0.12$ Å, both $A_y$ and $B_z$ are nonzero.

TABLE S5. Wave vector directions and atomic displacement patterns of the symmetry–adapted lattice modes that we use to specify the structural distortions of various $HfO_2$ phases. $O_1$ and $O_2$ are shown in Fig. S2. In the lower half of the table, we give the amplitudes of the modes in the calculated tetragonal, oIII and oIV structures. In the tetragonal structure, $X_2^-$ is the only non–zero mode. The oIII and oIV structures are generated by additional non–zero lattice modes amplitudes.

| | $\Gamma_{4,y}^-$ | $\Gamma_{4,z}^-$ | $X_2^-$ | $X_{5,x}^+$ | | $X_{5,y}^+$ | | $X_{5,z}^+$ | | $X_5^-$ |
|---|---|---|---|---|---|---|---|---|---|---|
| $\hat{\boldsymbol{q}}$ | $\mathbf{0}$ | $\mathbf{0}$ | $\hat{\boldsymbol{x}}$ | $\hat{\boldsymbol{y}}$ | $\hat{\boldsymbol{z}}$ | $\hat{\boldsymbol{x}}$ | $\hat{\boldsymbol{z}}$ | $\hat{\boldsymbol{x}}$ | $\hat{\boldsymbol{y}}$ | $\hat{\boldsymbol{z}}$ |
| Hf | $d_y$ | $d_z$ | 0 | 0 | 0 | 0 | 0 | 0 | 0 | 0 |
| $O_1$ | $-\frac{1}{2}d_y$ | $-\frac{1}{2}d_z$ | $-d_x$ | $d_x$ | $d_x$ | $-d_y$ | $d_y$ | $-d_z$ | $d_z$ | $d_y$ |
| $O_2$ | $-\frac{1}{2}d_y$ | $-\frac{1}{2}d_z$ | $-d_x$ | $d_x$ | $d_x$ | $d_y$ | $d_y$ | $d_z$ | $d_z$ | $-d_y$ |
| Amp. | $u_y$ | $u_z$ | | | | $A_y$ | $B_y$ | $A_z$ | $B_z$ | 0 |
| $Q_{\mathrm{t}}$ | 0 | 0 | 0.244 | 0 | 0 | 0 | 0 | 0 | 0 | 0 |
| $Q_{\mathrm{oIII}}$ | 0 | 0.236 | 0.471 | 0 | 0.389 | 0.405 | 0 | 0 | 0.398 | 0.115 |
| $Q_{\mathrm{oIV}}$ | 0.174 | 0.174 | 0.410 | 0 | 0 | 0.277 | 0 | 0.277 | 0 | 0 |

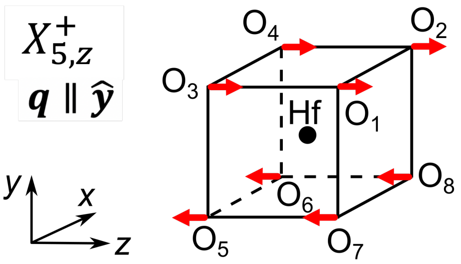


FIG. S2. Labeling of the atoms for the computation of the mode amplitudes, with the atomic displacement pattern shown for the $X_{5,z}^+$ ($\boldsymbol{q} \parallel \hat{\boldsymbol{y}}$) mode.

In this paragraph, we discuss how the amplitude of a specific mode is calculated for a given structure by projecting the atomic displacements in the structure onto the normalized atomic displacement pattern of the mode. We take $B_z$, the amplitude of the $X_{5,z}^+$ ($\boldsymbol{q} \parallel \hat{\boldsymbol{y}}$) mode, as our example. From Table S6, we find the atomic displacements for this mode are 0 for Hf, and $d_z$ for $O_1$ and $O_2$. Therefore, we only need to consider the atomic positions of

the oxygen atoms, and the expression for $B_z$ is

$$B_z = \frac{1}{4\sqrt{2}}(Z_{\mathrm{O1}} + Z_{\mathrm{O2}} + Z_{\mathrm{O3}} + Z_{\mathrm{O4}} - Z_{\mathrm{O5}} - Z_{\mathrm{O6}} - Z_{\mathrm{O7}} - Z_{\mathrm{O8}}), \tag{S1}$$

where $Z_{\mathrm{Oi}}$ is the $z$–component Cartesian coordinate of the oxygen atom i, as labeled is Fig. S2. Here, we note that $X_{5,z}^{+}$ $(\boldsymbol{q} \parallel \hat{\boldsymbol{y}})$ is a zone boundary mode with the wavevector $\boldsymbol{q} \parallel \hat{\boldsymbol{y}}$. Therefore, in the conventional 12–atom cell, the signs corresponding to O5–O8 should be different from those corresponding to O1–O4, since these two group of oxygen atoms are correlated by a translation along the $y$ axis. $\frac{1}{4\sqrt{2}}$ is the normalization factor, since 4 formula units are involved in the 12–atom cell and the normalization factor for each formula unit is $\frac{1}{\sqrt{2}}$.

## III. EFFECTIVE CHARGES AND CONSTRAINED RELAXATIONS

The effective charge used in electric field simulation is calculated as the average of the $yy$ and $zz$ components of the Born effective charge tensors in the tetragonal, oIII, and oIV phases (TABLE S1). We understand that the Born effective charges depend on the structure and chemical bonding environment. However, this approximation is reasonable, since the chemical bonds in $HfO_2$ based materials are primarily ionic, and the Born effective charges are not much different from the nominal ones. To calculate the Born effective charges of Y–$HfO_2$, we add one electron per Y atom, compensated by a uniform positive background, to make the system insulating.

TABLE S6. Effective charges of the atoms in different systems which we focus on in this study.

| | Hf | O | Y | Zr |
|---|---|---|---|---|
| $HfO_2$ | 5.305 | -2.653 | N/A | N/A |
| Y–$HfO_2$ | 5.287 | -2.568 | 4.072 | N/A |
| $Hf_{0.5}Zr_{0.5}O_2$ | 5.346 | -2.735 | N/A | 5.594 |

The constrained relaxation with fixed amplitudes of lattice modes are performed with the 'wtatcon' command in the ABINIT package. By using this command, the calculated forces $F_I$, are replaced by projected forces, $F_I^*$ to satisfy the constraint equation

$$\sum W_{i,I} F_{i,I}^* = 0 \tag{S2}$$

where $i = x, y, z$ and $I$ runs over all the atoms. For example, in order to fix amplitude of the polar $\Gamma_{4,y}^-$ mode, we need $W_{y,\mathrm{Hf}} = -2 \times W_{y,\mathrm{O}}$.

## IV. INTERMEDIATE STATES IN Y–HFO$_2$ AND HF$_{0.5}$ZR$_{0.5}$O$_2$

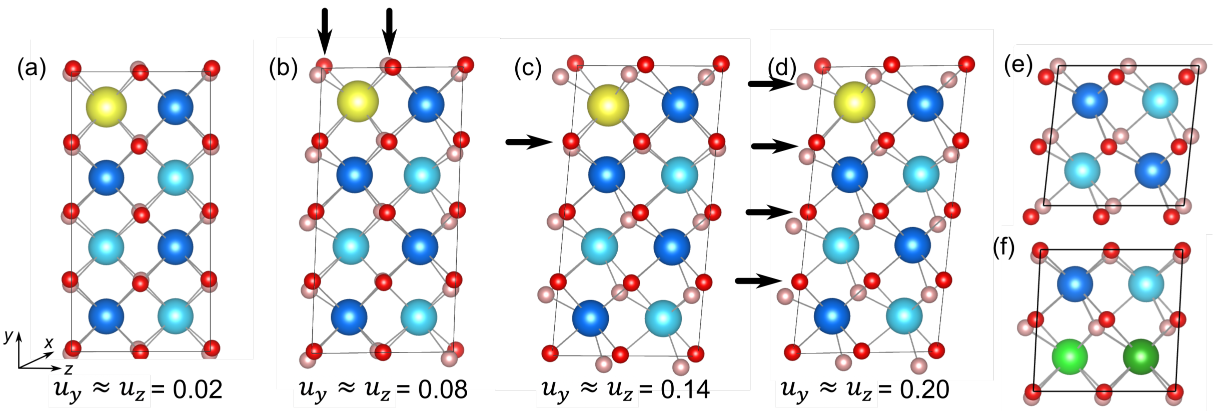


FIG. S3. (a)–(d) Representative Y–doped structures with $u = u_y = u_z = 0.02$, 0.08, 0.14 and 0.20 Å respectively. For $u < 0.04$ Å, the structure is quite similar to the tetragonal one. For $0.04 < u < 0.11$ Å, shown in (b), the distinctive feature of the intermediate state is that different columns of Hf atoms, indicated by the downward pointing arrows, have different displacements. For $0.11 < u < 0.16$ Å, shown in (c), the distinctive feature of the intermediate state is that one of the oxygen atom layers, indicated by the rightward pointing arrow, has approximately zero displacement. For $u > 0.16$ Å, shown in (d), the structure is in the oIV phase. Due to the Y doping, the four different layers of oxygen atoms have slightly different displacements, leading to a non–zero $B_z$. (e) In the oIV phase of pure $HfO_2$, oxygen atoms in different layers are equally displaced, leading to a zero $B_z$. (f) In $Hf_{0.5}Zr_{0.5}O_2$, the symmetry is broken due to Zr substitutions. The oxygen atoms have different displacements in adjacent layers, leading to a non–zero $B_z$.

## V. EVOLUTION OF THE ENERGY LANDSCAPES UNDER ELECTRIC FIELD

As discussed in the main text, electrical enthalpy $H = U - E \cdot P$ is used to describe the change of phase stability under electric field $E$. Here, $U$ is the zero–field energy. $P$ is the polarization computed using the linear approximation, and therefore is proportional to the amplitude of the polar mode. The hysteresis loops are calculated with the finite electric field method and identical with ones in the main text. Here, we note that the position of a point given by the electrical enthalpy profile may deviate from the hysteresis loops a little bit, which is attributed to the estimation of polarization with the linear approximation method. In the following figures, we move the points to align with the hysteresis loops for a clearer view.

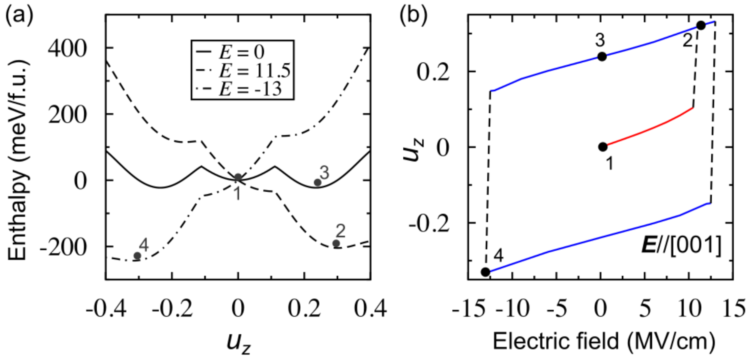


FIG. S4. (a) Enthalpy profile of pure $HfO_2$ under electric fields along the [001] direction; (b) computed polarization–field hysteresis presented in the main text. Point 1: the initial structure is non–polar tetragonal; Point 2: for $E = 11.5$ MV/cm, the local minimum near $P = 0$ disappears and the structure transforms to the oIII one; Point 3: after the electric field is removed, the structures remains oIII; Point 4: for $E = -13$ MV/cm, the positive $P$ minimum disappears and the polarization flips.

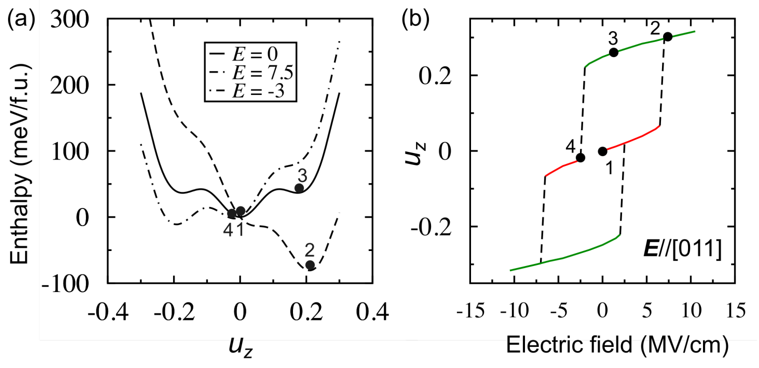


FIG. S5. (a) Enthalpy profile of pure $HfO_2$ under electric fields along the [011] direction; (b) computed $P$–$E$ hysteresis. Point 1: the initial structure is non–polar tetragonal; Point 2: for $E = 7.5$ MV/cm, the local minimum near $P = 0$ disappears and the structure transforms to oIV; Point 3: after the electric field is removed, the structure remains oIV; Point 4: for $E = -3$ MV/cm, the large $P$ minimum disappears and the system returns to the local minimum corresponding to the tetragonal structure.

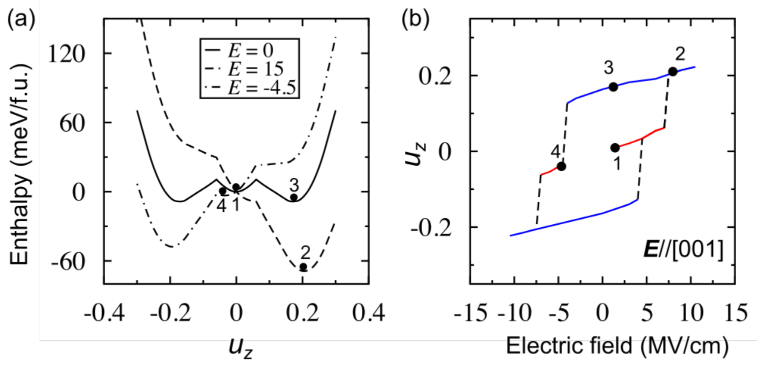


FIG. S6. (a) Enthalpy profile of Y–$HfO_2$ under electric fields along the [001] direction; (b) computed $P$–$E$ hysteresis. Point 1: the initial structure is non–polar tetragonal; Point 2: for $E = 7.5$ MV/cm, the local minimum near $P = 0$ disappears and the structure transforms to oIII; Point 3: after the electric field is removed, the structure remains oIII; Point 4: for $E = -4.5$ MV/cm, the large $P$ minimum disappears and the system returns to the minimum corresponding to the t–phase.

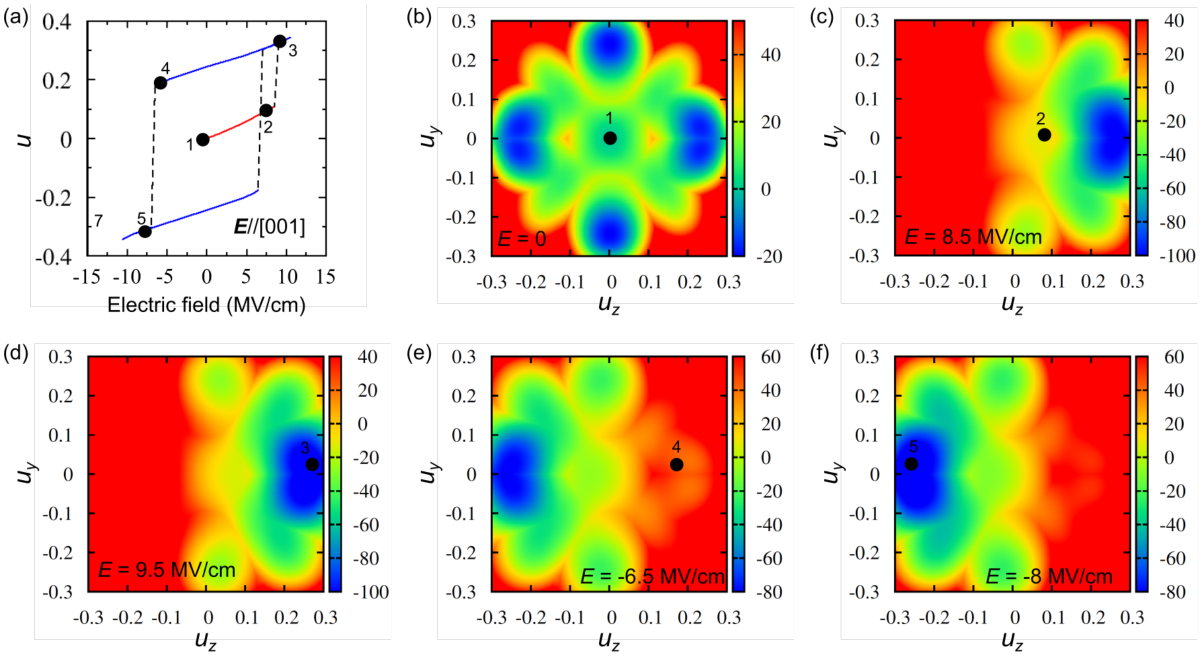


FIG. S7. (a) Computed polarization–field hysteresis loop presented in the main text; (b)–(f) enthalpy landscape of $Hf_{0.5}Zr_{0.5}O_2$ under electric fields along the [001] direction; Point 1: $E = 0$, the initial structure is non–polar tetragonal [subfigure (b)]; Point 2: $E = 8.5$ MV/cm, the state moves toward the local minimum corresponding to the oIII structure, but is blocked by the arrow–shape energy barrier [subfigure (c)]; Point 3: $E = 9.5$ MV/cm, the structure transforms to oIII [subfigure (d)]; Point 4: $E = -6.5$ MV/cm, the system is trapped in the oIII local minimum [subfigure (e)]; Point 5: $E = -8$ MV/cm, the positive $P$ minimum disappears and the polarization flips [subfigure (f)].

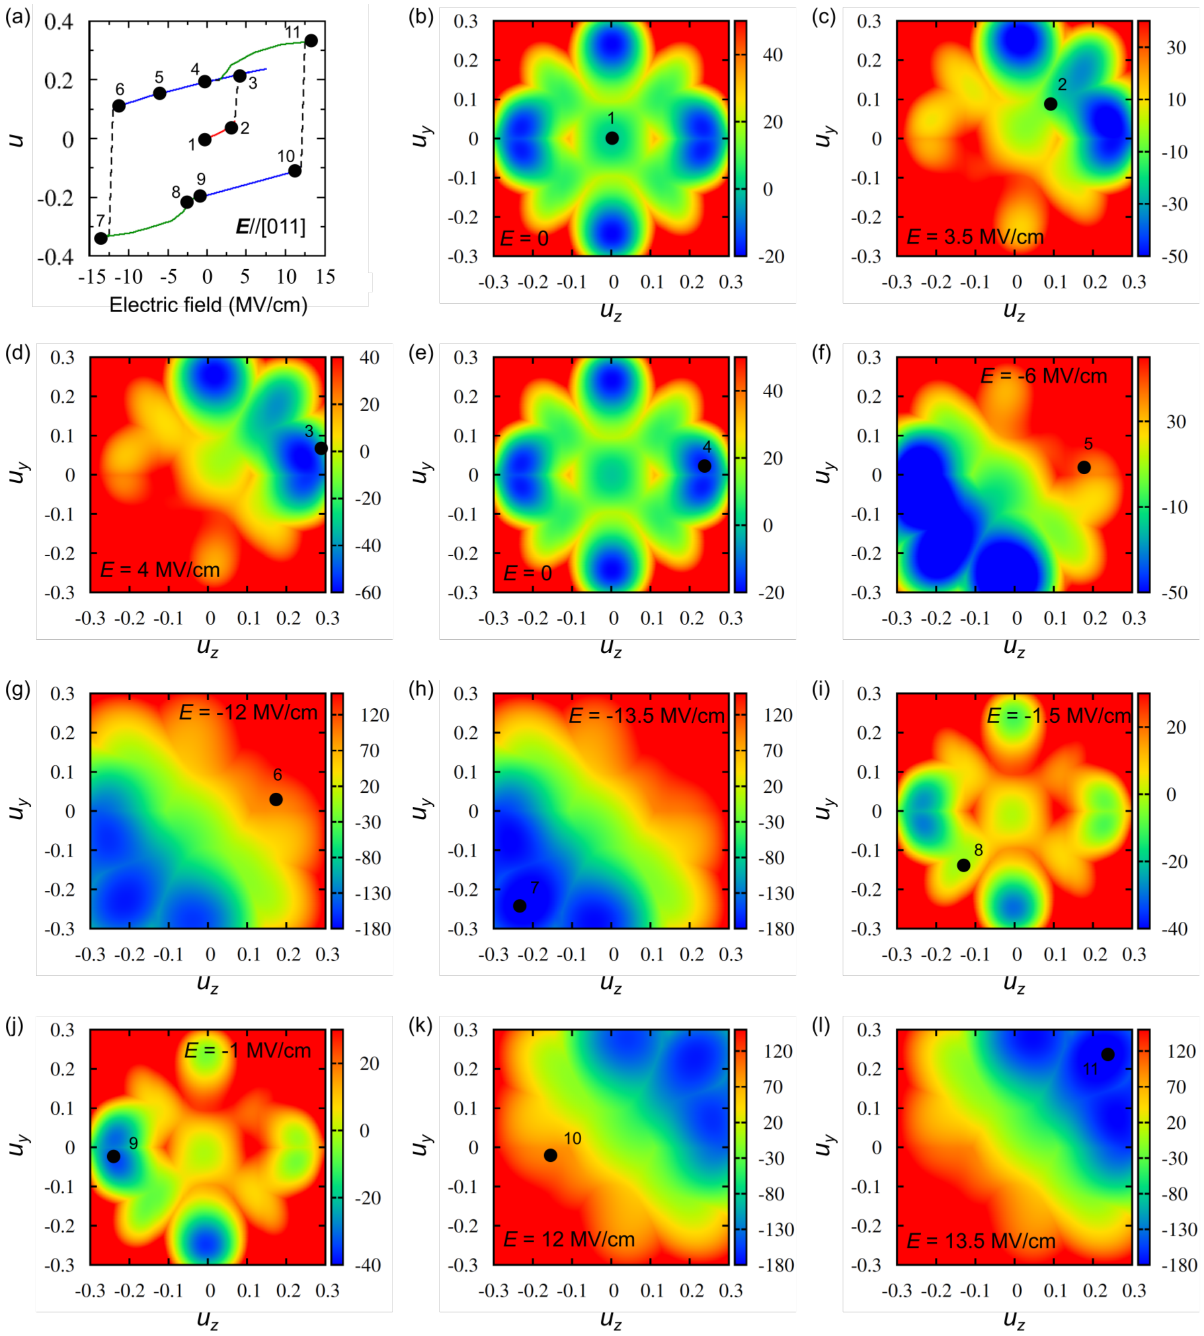


FIG. S8. (a) Computed $P$–$E$ loop; (b)–(l) enthalpy landscape of $Hf_{0.5}Zr_{0.5}O_2$ under electric fields along the [011] direction. The state starts from the local minimum corresponding to the tetragonal structure [(b)], and moves toward the [011]–polarized oIV structure [subfigure (b)] under electric field [$E$ = 3.5 MV/cm, (c)]. However, the oIV structure is unstable, and the state falls into the local minimum corresponding to the [001]–polarized oIII structure [$E$ = 8 MV/cm, (d)]. Next, a large reverse electric field ($E > -13.5$ MV/cm) is required to drive the state out of this local minimum [(e)–(h)]. Under this electric field, the polarization switches to the [0$\bar{1}\bar{1}$]–polarized oIV phase [(h) and (i)]. Then the magnitude of the electric field is reduced, once it reaches -1 MV/cm, the oIV structure becomes unstable again and the system collapses to the [00$\bar{1}$]–polarized oIII one

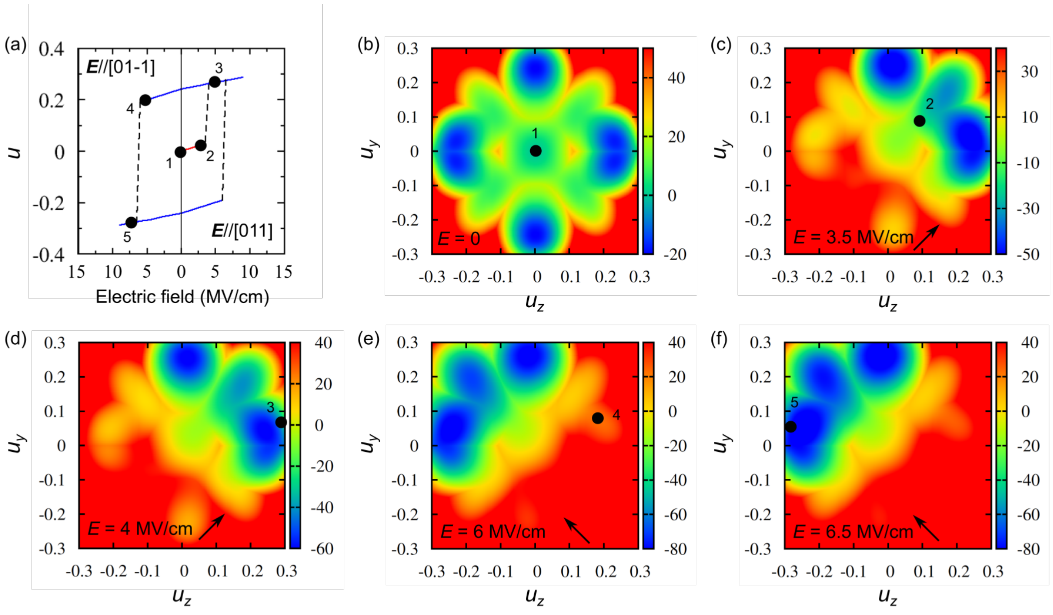


FIG. S9. (a) Computed hysteresis loop; (b)–(f) enthalpy landscape of $Hf_{0.5}Zr_{0.5}O_2$. To keep the state on the track of the optimal path, forward $E$ is along the [011] direction and the backward $E$ is along $[01\bar{1}]$. Point 1: At $E = 0$, the structure is non–polar tetragonal [subfigure (b)]; Point 2: $E = 3.5$ MV/cm. As the magnitude of $E$ increases from zero, the polarization increases along the [011]–direction and the structure moves toward the [011]–polarized oIV structure [subfigure (c)]; Point 3: $E = 4$ MV/cm. Since at this field the oIV structure is unstable, the structure transforms to the [001]–polarized oIII one [subfigure (d)]; Point 4: Here, we flip the $z$ component of the electric field and it becomes $[01\bar{1}]$ directed. For $E < 6$ MV/cm, the structure is trapped in the local minimum corresponding to [001]–polarized oIII structure [subfigure (e)]; Point 5: $E = 6.5$ MV/cm. As the magnitude of the field increases, the polarization along the $z$–direction flips and the state goes to the $[00\bar{1}]$–polarized oIII local minimum [subfigure (f)].

---

[S1] S. E. Reyes-Lillo, K. F. Garrity, and K. M. Rabe, Phys. Rev. B **90**, 140103 (2014).

[S2] X. Zhao and D. Vanderbilt, Phys. Rev. B **65**, 233106 (2002).

[S3] A. A. Demkov, Phys. Status Solidi B **226**, 57 (2001).

[S4] T. D. Huan, V. Sharma, G. A. Rossetti Jr, and R. Ramprasad, Phys. Rev. B **90**, 064111 (2014).
